# Supplementary material for: Search for $\mathrm{GeV}$-scale axion-like particles in PbPb collisions
Source: arXiv:2611.00135 source file (2026-11-03)
Supplement: Supplementary file 1 [file appendix.tex]

% ===============================================================================
% Purpose: appendix to the standard template: standard symbol alises from Ulrik
% Author: Tomasz Skwarnicki
% Created on: 2009-09-24
% ===============================================================================

%{\noindent\normalfont\bfseries\Large Appendices}
\section*{Appendices}

\appendix

\section{Standard References}
\label{sec:StandardReferences}
a

%%%%%%%%%%%%%%%%%%%%%%%%%%%%%%%%%%
